# Supplementary material for: Revisiting Self-Training for Few-Shot Learning of Language Model
Source: arXiv:2110.01256 source file (2021-10-04)
Supplement: Supplementary file 1 [file appendix.tex]

\appendix

\section{Datasets}
\label{sec:datasets}

For SNLI~\citep{Bowman2015ALA}, and GLUE datasets~\citep{Wang2018GLUEAM}, including SST-2~\cite{socher-etal-2013-recursive}, MNLI~\citep{williams-etal-2018-broad}, QNLI~\citep{rajpurkar-etal-2016-squad}, RTE~\citep{10.1007/11736790_9, haim2006second, giampiccolo-etal-2007-third,bentivogli2009fifth}, MRPC~\citep{dolan-brockett-2005-automatically}, we follow \citet{Zhang2020RevisitingFB} to take original development set as test set. For, other single sentence tasks, MR~\citep{pang-lee-2005-seeing}, CR~\citep{hu2004mining}, MPQA~\citep{wiebe2005annotating}, Subj~\citep{pang-lee-2004-sentimental}, we use the same train-test split as \citep{gao2020making}. For SST-5~\citep{socher-etal-2013-recursive}, we use the official test sets. Dataset descriptions and prompt we used are summarized in Table .
